# Supplementary material for: Model-Protected Multi-Task Learning
Source: arXiv:1809.06546 source file (2019-07-02)
Supplement: Supplementary file 2 [file appendix_in_main.tex]

\appendices
\section{Wishart Distribution}\label{sec:df_wishart}
%In this paper, the Wishart distribution will be used, which is defined below.
\begin{definition}[\citet{gupta1999matrix}]
A $d \times d$ random symmetric positive definite matrix $\E$ is said to have a
Wishart distribution $\E\sim W_d(\V,\nu)$ if its probability density function is
\begin{equation*}
  p(\E) = \frac{|\E|^{(\nu-d-1)/2}\exp(-\rm tr(\V^{-1}\E)/2)}{2^{\frac{\nu d}{2}}|\V|^{1/2}\Gamma_d(\nu/2)},
\end{equation*}
where $\nu > d-1$ and $\V$ is a $d \times d$ positive definite matrix.
\end{definition}
